# Supplementary material for: Asymptotic properties of Principal Component Analysis and shrinkage-bias adjustment under the Generalized Spiked Population model
Source: arXiv:1607.08647 source file (2016-07-28)
Supplement: Supplementary file 1 [file suppA.pdf]

# SUPPLEMENT A: SUPPLEMENTARY TABLES AND FIGURES FOR “ASYMPTOTIC PROPERTIES OF PRINCIPAL COMPONENT ANALYSIS AND SHRINKAGE-BIAS ADJUSTMENT UNDER THE GENERALIZED SPIKED POPULATION MODEL”

BY ROUNAK DEY AND SEUNGGEUN LEE

*Department of Biostatistics, University of Michigan*

Some additional tables and figures that were referred to in “Asymptotic properties of Principal Component Analysis and shrinkage-bias adjustment under the Generalized Spiked Population model” are provided in this supplementary material.

TABLE 1  
Number of simulated datasets (out of 200) where the number of distant spikes were estimated to be 1, 2, 3 or  $\geq 4$

| Settings |     |       |            |        | Estimated no. of distant spikes |     |    |          |
|----------|-----|-------|------------|--------|---------------------------------|-----|----|----------|
| No.      | $n$ | $p$   | $\sigma^2$ | $\rho$ | 1                               | 2   | 3  | $\geq 4$ |
| 1        | 500 | 5000  | 4          | 0.8    | 0                               | 77  | 77 | 46       |
| 2        | 500 | 5000  | 1          | 0.7    | 0                               | 139 | 53 | 8        |
| 3        | 500 | 5000  | 7.5        | 0.8    | 95                              | 78  | 20 | 7        |
| 4        | 500 | 5000  | 4          | 0      | 0                               | 188 | 12 | 0        |
| 5        | 500 | 50000 | 4          | 0.8    | 0                               | 167 | 30 | 3        |

Fig 1: Linkage disequilibrium

Hapmap III CEU+TSI samples, 848 SNPs on Chr. 9, created using Haploview (Barrett et al., 2005)

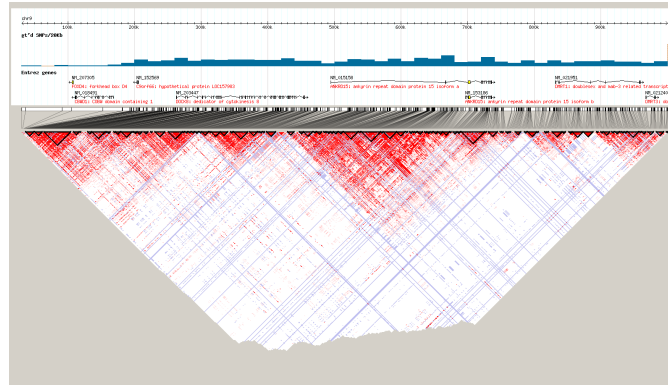

Fig 2: Sample sizes of the test samples that were included in the prediction error estimation for different values of the thresholding parameter  $\epsilon$

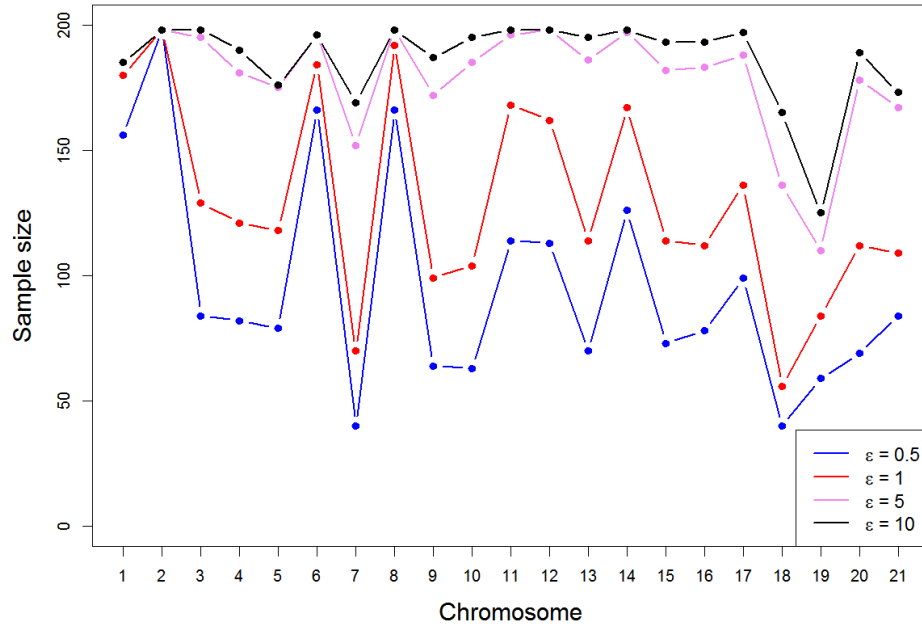

Fig 3: Distribution of the number of markers across different chromosomes

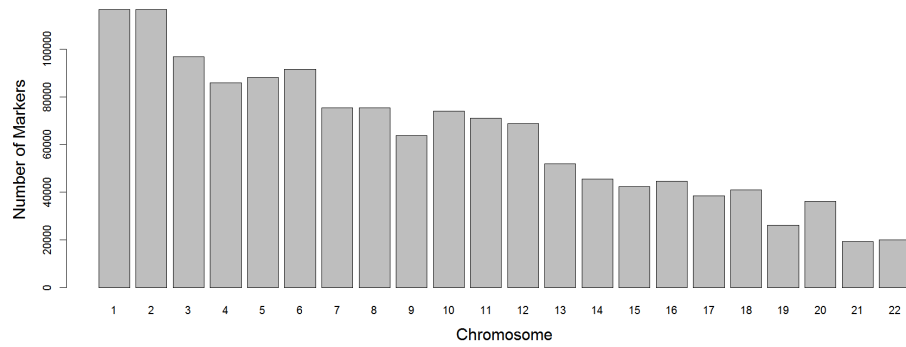

Fig 4: Comparison of the mean squared errors (MSE) of the unadjusted and adjusted PC scores based on the  $d$ -GSP and SP methods with the adjusted PC scores based on the  $\lambda$ -GSP method. The ratios of the MSEs are presented for chromosome 1-21 using different values of the thresholding parameter  $\epsilon$ . The Y-Axis is presented in a logarithmic scale.

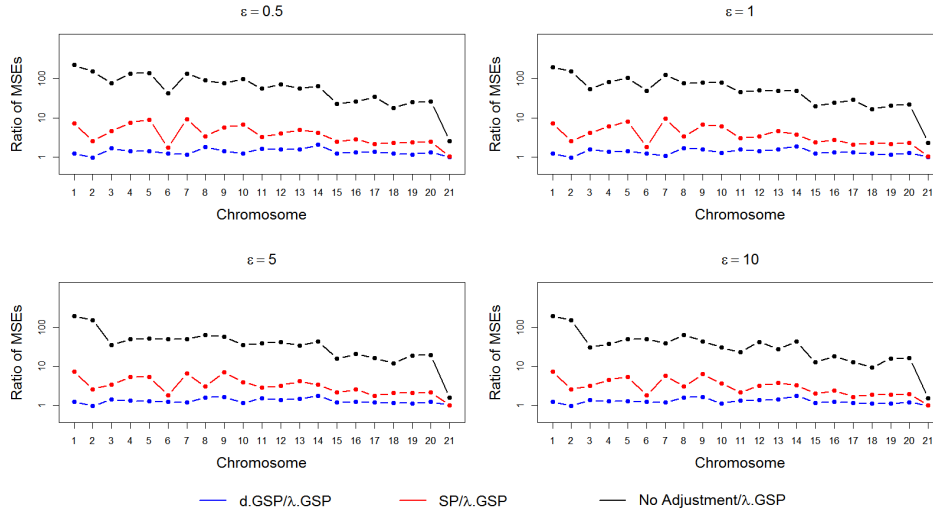

**References.**

BARRETT, J. C., FRY, B., MALLER, J. and DALY, M. J. (2005). Haploview: analysis and visualization of LD and haplotype maps. *Bioinformatics* **21** 263-265.

DEPARTMENT OF BIostatISTICS  
UNIVERSITY OF MICHIGAN SCHOOL OF PUBLIC HEALTH  
1415 WASHINGTON HEIGHTS  
ANN ARBOR, MI 48109-2029, USA  
E-MAIL: [deyrnk@umich.edu](mailto:deyrnk@umich.edu)  
[leeshawn@umich.edu](mailto:leeshawn@umich.edu)
